# Supplementary material for: A Transferable Approach for Partitioning Machine Learning Models on Multi-Chip-Modules
Source: arXiv:2112.04041 source file (2021-12-07)
Supplement: Supplementary file 1 [file appendix.tex]

\appendix

\section{Appendix}

Optionally include extra information (complete proofs, additional experiments and plots) in the appendix.
This section will often be part of the supplemental material.
